# Supplementary material for: Local stress tensor calculation by the Method-of-Plane in microscopic systems with macroscopic flow: a formulation based on the velocity distribution function
Source: arXiv:2107.07785 source file (2021-07-16)
Supplement: Supplementary file 1 [file appendix.tex]

\section{
%Evaluation wall-tangential velocity on bins
%parallel to the wall.
\yy{
Possible extension of the present VDF-based 
average 
%for the calculation of 
to the interaction-induced stress
defined on the to MoP plane.
}
\label{secapp:Vx_on_xandz}
}
\begin{figure}[h]
  \begin{center}
    \includegraphics[width=0.7\linewidth]{./fig5.eps}
  \end{center} 
  \caption{\label{fig:fig5}
%   (a) Distributions of the macroscopic velocity in the $x$-direction $v_{x}(S_{x})$ and $v_{x}(S_{z})$ calculated at $x$-normal, and $z$-normal bin faces by Eqs. \eqref{eq:vxSx} and \eqref{eq:vxSz}, respectively. The $z$-positions of $v_{x}(S_{x})$ and $v_{x}(S_{z})$ are defined at the center of the bin face.
  (b) Distributions of the diagonal stress and advection components $\tau_{xx}$, $\tau_{xx}-\rho U_{x}U_{x}$ and $\tau_{yy}-\rho U_{y}U_{y}$ calculated at the same $x$-normal bin face.
% (a)Comparison of mean velocity in $x$-direction calculated at $x-$normal, and $z-$normal planes defined by Eqs. \eqref{eq:Uxx} and \eqref{eq:Uxz}, respectively. 
% (b) Distributions of the diagonal stress components $\tau_{xx}$, $\tau_{zz}$ and the advection term in $x$-direction  $\rho U_{x}U_{x}$.
% (c) The comparison of the off-diagonal stress components $\tau_{xz}$ and $\tau_{zx}$ calculated on $x-$normal, and $z-$normal planes, respectively.
}
\end{figure}
\yy{
As shown in Fig.~\ref{fig:fig2}, 
the velocity (and density) can be properly calculated based on the VDF-based average.
%As same as the mass flux and the velocity, all the stress components can be calculated at a bin face with arbitrary normal vector. 
Here, we propose a possible extension of this idea to the calculation of the interaction interaction-induced stress $\tau^\mathrm{int}$ 
defined on an arbitrary bin face, and we show a comparison in the system in Fig.~\ref{fig:fig1}.
}
diagonal stress and the advection term $\tau_{xx}$, $\tau_{yy}$, $\rho v_{x} v_{x}$ and $\rho v_{y} v_{y}$ \yy{in the system in Fig.~\ref{fig:fig1}}.
The kinetic term of $\tau_{yy}(S_{x})-\rho v_{y} v_{y}(S_{x})$ is defined by using Eq.~\eqref{eq:sigmasum} as 
\begin{align}
%\nonumber
\tau^{\text{kin}}_{yy}(S_{x})-\rho v_{y} v_{y}(S_{x})
&=
-\lim_{\delta t \to 0}\frac{1}{S_{x}\delta t}\left<
\sum_{i\in\mathrm{fluid},\delta t}^{\text{crossing } S_{x}}
\frac{mu_{y}^{i}u_{y}^{i}}{\left| u_{x}^{i}\right|}
\right>.
\end{align}
Considering that there is no flow in the $y$-direction, \ie \yy{$v_{y}=0$}, it follows
\begin{align}
%\nonumber
\tau^{\text{kin}}_{yy}(S_{x})
%-\rho v_{y} v_{y}(S_{x})
&=
-\lim_{\delta t \to 0}\frac{1}{S_{x}\delta t}\left<
\sum_{i\in\mathrm{fluid},\delta t}^{\text{crossing } S_{x}}
\frac{mu_{y}^{i}u_{y}^{i}}{\left| u_{x}^{i}\right|}
\right>.
\end{align}
The two diagonal stress components $\tau_{xx}$ and $\tau_{yy}$ should agree well \yy{in this quasi-1D steady state system with all macroscopic physical properties given as a unique function of $z$. 
}
$\tau_{xx}$ and $\tau_{yy}-\rho v_{y} v_{y}$ should be equal.

%\rem{because of the system symmetry}. %because the wall-tangential normal stress consists of the pressure and the solid-liquid interfacial tension.

%
The interaction term $\tau^{\text{int}}_{yy}$ is also calculated at the $x$-normal bin face same as the kinetic term by changing the numerator of the fraction of the Eq.~\eqref{eq:stress_int} as
\begin{align}
    \tau_{yy}^\mathrm{int}(S_{x})=
    -\frac{1}{S_{x}}
    \angb{
    \sum_{(i,j)\in \mathrm{fluid}}^{\text{across\ } S_{x}} 
    F^{ij}_{y} \frac{r^{ij}_{y}}{|r^{ij}_{x}|}
    },
\end{align}
because the denominator denotes the weighted average corresponding to the calculation bin face.
Figure~\ref{fig:fig5} shows the distributions of the stress and the advection term $\tau_{xx}$, $\tau_{xx}-\rho v_{x} v_{x}$ and  $\tau_{yy}-\rho v_{y} v_{y}$.
\yy{The latter two} 
%$\tau_{xx}$ and $\tau_{yy}-\rho v_{y} v_{y}$
%starting a sentence with a symbol (number, abbreviation too) is not preferred.
%$\tau_{yy}-\rho v_{y} v_{y}$ and $\tau_{xx}$ 
agreed well, indicating that the extraction of $\tau_{yy}-\rho v_{y} v_{y}$ by the $x$-normal bin face is possible.
